# Supplementary material for: Search for new phenomena in high-mass diphoton final states using 37 fb$^{-1}$ of proton-proton collisions collected at $\sqrt{s}=13$ TeV with the ATLAS detector
Source: arXiv:1707.04147 source file (2017-12-19)
Supplement: Supplementary file 1 [file appendix.tex]

\part*{Auxiliary material}
\addcontentsline{toc}{part}{Auxiliary material}

\begin{figure}[!ht]
\centering
    \includegraphics[width=1.0\columnwidth]{figures/aux/JiveXML_309516_3908489606-2p6_1GeVIndetCut.pdf}
    \caption{Event display of the highest-invariant-mass ($m_{\gamma\gamma}=2.57$~\TeV) diphoton candidate event selected in data.
      The event passes both the spin-0 selection and the spin-2 selection.
      Only inner-detector tracks with $\pt>5$~\GeV, calorimeter cells with transverse energy deposits larger than 1~\GeV\ and
      cells of the tile hadronic calorimeter with transverse energy above 3~\GeV\ are shown.
      Both photon candidates are reconstructed as unconverted.
      The leading photon candidate has $\ET=1345$~\GeV, $\eta=-0.09$, $\phi=-2.42$, $\ETiso = -0.15$~\GeV.
      The subleading photon candidate has $\ET=1227$~\GeV, $\eta=-0.06$, $\phi=0.69$, $\ETiso = 2.29$~\GeV.}
    \label{fig:evt_display_a}
\end{figure}

\begin{figure}[!ht]
\centering
    \includegraphics[width=1.0\columnwidth]{figures/aux/JiveXML_303291_327585180-2p45_1GeVIndetCut.pdf}
    \caption{Event display of the second-highest-invariant-mass ($m_{\gamma\gamma}=2.45$~\TeV) diphoton candidate event selected in data.
      The event passes the spin-2 selection but not the spin-0 selection.
      Only inner-detector tracks with $\pt>5$~\GeV, calorimeter cells with transverse energy deposits larger than 1~\GeV\ and
      cells of the tile hadronic calorimeter with transverse energy above 3~\GeV\ are shown.
      The leading photon candidate is reconstructed as converted and has $\ET=443$~\GeV, $\eta=2.24$, $\phi=-2.14$, $\ETiso = -1.32$~\GeV.
      The subleading photon candidate is reconstructed as unconverted and has $\ET=412$~\GeV, $\eta=-1.18$, $\phi=-0.96$, $\ETiso = -0.32$~\GeV.}
    \label{fig:evt_display_b}
\end{figure}

\FloatBarrier

\begin{figure}[!h]
  \begin{center}
    \subfloat[]{\includegraphics[width=.5\textwidth]{figures/aux/resolution_spin0_800GeV_nwa.pdf}}
    \subfloat[]{\includegraphics[width=.5\textwidth]{figures/aux/resolution_spin0_800GeV_Gamma06.pdf}}\\
    \subfloat[]{\includegraphics[width=.5\textwidth]{figures/aux/resolution_spin2_1000_kappa01.pdf}}
    \subfloat[]{\includegraphics[width=.5\textwidth]{figures/aux/resolution_spin2_1000_kappa2.pdf}} 
\end{center}
  \caption{The normalized $m_{\gamma\gamma}$ distributions for different signal hypotheses
    for a scalar resonance with a mass of 800~\GeV,
    and (a) with a narrow decay width and (b) with relative width $\Gamma_{X}/m_{X}$ = 0.06,
    and for a KK graviton predicted by the RS1 model with a mass of 1000~\GeV,
    and (c) with \coupling\ = 0.01 and (d) with \coupling\ = 0.2.
    In all cases, a parameterized signal model is superimposed using the convolution of the signal mass
    line-shape with the overall detector resolution.}
\label{fig:dscb_fit}
\end{figure}

\begin{figure}[!h]
\begin{center}
  \subfloat[]{\includegraphics[width=.49\textwidth]{figures/aux/mass_spin0_2015_bkg}}
  \subfloat[]{\includegraphics[width=.49\textwidth]{figures/aux/mass_spin2_2015_bkg}}  
\end{center}
\caption{Distributions of the diphoton invariant-mass for events from 2015 data passing (a) the spin-0 or (b) the spin-2 selection,
  with the background-only fits superimposed. The differences between the data and the fits are shown in the bottom panels.
  The arrows in the lower panels indicate values outside the range by more than one standard deviation.
  There is no data event with $m_{\gamma\gamma}>2000$~\GeV.
}
\label{fig:mgg_distributions2015}
\end{figure}

\begin{figure}[!h]
\begin{center}
  \subfloat[]{\includegraphics[width=.49\textwidth]{figures/aux/mass_spin0_2016_bkg}}
  \subfloat[]{\includegraphics[width=.49\textwidth]{figures/aux/mass_spin2_2016_bkg}}  
\end{center}
\caption{Distributions of the diphoton invariant-mass for events from 2016 data passing (a) the spin-0 or (b) the spin-2 selection,
  with the background-only fits superimposed. The differences between the data and the fits are shown in the bottom panels.
  The arrows in the lower panels indicate values outside the range by more than one standard deviation.
  There is no data event with $m_{\gamma\gamma}>2700$~\GeV. 
}
\label{fig:mgg_distributions2016}
\end{figure}

\begin{figure}[h]
\begin{center}
\subfloat[]{\includegraphics[width=.5\textwidth]{figures/aux/1dp0_spin0_0}}
\subfloat[]{\includegraphics[width=.5\textwidth]{figures/aux/1dp0_spin0_0_02}} \\
\subfloat[]{\includegraphics[width=.5\textwidth]{figures/aux/1dp0_spin0_0_06}}
\subfloat[]{\includegraphics[width=.5\textwidth]{figures/aux/1dp0_spin0_0_10}}
\end{center}
   \caption{Compatibility with the background-only hypothesis as a function of the assumed signal mass $m_X$ 
for different values of the relative width $\Gamma_X/m_X$ from the spin-0 resonance search.}
\label{fig:1dp0_spin0}
\end{figure}

\begin{figure}[h]
\begin{center}
\subfloat[]{\includegraphics[width=.5\textwidth]{figures/aux/1dp0_spin2_0_01}}
\subfloat[]{\includegraphics[width=.5\textwidth]{figures/aux/1dp0_spin2_0_10}} \\
\subfloat[]{\includegraphics[width=.5\textwidth]{figures/aux/1dp0_spin2_0_20}}
\subfloat[]{\includegraphics[width=.5\textwidth]{figures/aux/1dp0_spin2_0_30}}
\end{center}
   \caption{Compatibility with the background-only hypothesis as a function of the assumed  mass of the KK graviton predicted by the RS1 model,
for different values of \coupling\ from the spin-2 resonance search.}
\label{fig:1dp0_spin2}
\end{figure}

\begin{figure}[!h]
\begin{center}
\subfloat[]{\includegraphics[width=.5\textwidth]{figures/aux/acceptance_efficiency_spin0.pdf}}
\subfloat[]{\includegraphics[width=.5\textwidth]{figures/aux/acceptance_efficiency_spin2.pdf}}\\
\subfloat[]{\includegraphics[width=.5\textwidth]{figures/aux/acceptance_efficiency_add.pdf}}
\end{center}
 \caption{Fiducial acceptance (full points) and product of the fiducial acceptance times the combined reconstruction and identification efficiency (``Detector selection'', open points)
   as a function of the mass 
   for (a) a spin-0 resonant signal with narrow width under the spin-0 selection,
   (b) a \mbox{spin-2} resonant signal with $\coupling=0.1$ under the spin-2 selection, and
   (c) an ADD excess (GRW formalism), calculated as the difference between the sum of ADD and SM contributions (including their interference) and the SM contribution, under the spin-2 selection in the signal region $\mgg>2240$~\GeV.
   For larger values of \ms, the acceptance decreases to about 58\% at 8~\TeV\ due to a larger contribution from the interference term, which has smaller acceptance.
   The definition of fiducial region used for (a) is provided in the Letter text.
   The definition used for (b) is provided in JHEP 09 (2016) 001,
   and $\mgg>2240$~\GeV is required in addition for (c).
   Only MC statistical uncertainties are included.
 }
\label{fig:acceptance_efficiency}
\end{figure}

\begin{figure}[h]
\begin{center}
\subfloat[]{\includegraphics[width=.5\textwidth]{figures/aux/limit_spin0_0_02}} \\
\subfloat[]{\includegraphics[width=.5\textwidth]{figures/aux/limit_spin0_0_06}}
\subfloat[]{\includegraphics[width=.5\textwidth]{figures/aux/limit_spin0_0_10}}
\end{center}
\caption{Upper limits, calculated using the asymptotic approximation, on the fiducial cross section of a spin-0 particle at $\sqrt{s} = 13$~\TeV\ times branching ratio to two photons as a function of the assumed mass $m_X$, 
for different
values of the decay width divided by the mass. 
}
\label{fig:spin0_limit}
\end{figure}

\begin{figure}[h]
\begin{center}
\subfloat[]{\includegraphics[width=.5\textwidth]{figures/aux/limit_spin2_0_01}}\\
\subfloat[]{\includegraphics[width=.5\textwidth]{figures/aux/limit_spin2_0_20}}
\subfloat[]{\includegraphics[width=.5\textwidth]{figures/aux/limit_spin2_0_30}}
\end{center}
\caption{Upper limits, calculated using the asymptotic approximation, on the production cross section of a KK graviton at $\sqrt{s} = 13$~\TeV\ times branching ratio to two photons as a function of the assumed mass, for different
values of \coupling. 
The predicted cross sections times branching ratio to two photons in the RS1 model, computed at LO, are also shown. The uncertainty
in the cross-section values represents the PDF uncertainty.
}
\label{fig:spin2_limit}
\end{figure}

\begin{figure}[hbtp]
\centering
\includegraphics[width=.8\textwidth]{figures/aux/data_bkg_ADD_B_M} 
\caption{
  Observed invariant-mass distribution of diphoton events from the spin-2 selection, 
  with the predicted SM background and expected signals for one KK graviton predicted by the RS1 model with $\mG=4~\TeV$,
  as well as two values of the ADD model (GRW formalism) parameter \ms\ (3.5~\TeV, 6~\TeV) superimposed.
  The vertical dashed line and the arrow indicate the signal region of $\mgg>2240$~\GeV where the counting experiment is performed for the spin-2 non-resonant signal search.
}
\label{fig:bkgADD}
\end{figure}

\begin{figure}[hbtp]
\centering
\includegraphics[width=.8\textwidth]{figures/aux/ADD_Limits_with_Kfactor}
\caption{95\% CL upper limits on the number of excess events as a function of the ADD model (GRW formalism) parameter \ms. The black horizontal line corresponds to the observed limit, the dashed line corresponds to the expected limit and the green (yellow) band to the $\pm 1\sigma$ ($\pm 2\sigma$) uncertainty in the expected limit. The red curve corresponds to MC predictions from samples with different \ms\ values
  with the K-factor applied.
  The band around it illustrates the PDF and scale uncertainties in the signal. When the prediction is greater than the limit line, the corresponding value of \ms\ is excluded.
}
\label{fig:limitADD}
\end{figure}

\begin{figure}[hbtp]
\centering
\includegraphics[width=.8\textwidth]{figures/aux/bkg_systematics_summary_spin2.pdf} 
\caption{Relative pre-fit uncertainties in the shape of the \mgg\ distribution of the predicted background for the spin-2 resonance and non-resonant searches. The uncertainties are shown in the mass range 200~\GeV\ to 5000~\GeV, which is corresponding to the range where the signal-plus-background fit is performed in the resonance search. The reducible background uncertainty corresponds to the uncertainty in the shape of the reducible background component. The uncertainty in the shape of the irreducible background results from uncertainties affecting the NLO diphoton computation (parton distribution functions and factorization and renormalization scales). The uncertainty in the purity corresponds to the impact of the relative normalization of the reducible background compared to the irreducible background. The uncertainty in isolation results from the uncertainty due to the choice of parton-level isolation cut in the \textsc{Diphox} NLO computation.}
\label{fig:spin_2_syst_summary}
\end{figure}

\begin{figure}[hbpt]
\centering
\includegraphics[width=0.8\columnwidth]{figures/aux/DiphoxSherpa}
\caption{Effective $k$-factor correction as a function of diphoton mass obtained from the ratio \textsc{Diphox}/\textsc{Sherpa} at truth level for the irreducible background estimation used in the spin-2 searches.
  To focus on the shape comparison, the histogram has been normalized in such a way that that the integral of the ratio in the region 200--300~\GeV\ is equal to unity.
  The solid line represents the result of a fit to a smooth function.
}
\label{fig:BkgkFactor}
\end{figure}

\begin{figure}[hbpt]
\centering
\subfloat[]{\includegraphics[width=0.48\columnwidth]{figures/aux/GravitonAnal_LeadFinal.pdf}}
\subfloat[]{\includegraphics[width=0.48\columnwidth]{figures/aux/GravitonAnal_SubLeadFinal.pdf}}
\caption{Modified isolation energies $\ETisomod = \ETiso - 0.022\et$ for (a) the leading and (b) the subleading photon candidate for events selected in the low-mass control region ($200\, \GeV < \mgg < 510\, \GeV$) of the spin-2 analyses.
  The result of the two-dimensional template fit, used for the determination of the background composition in the spin-2 searches, is shown in black, together with the contributions of the different jet (green lines) and photon (red lines) components.
  The bin-by-bin significance of the difference between data and the fit is shown in the bottom panels.
}
\label{fig:Fit2D}
\end{figure}

\begin{table}
  \centering
  \begin{tabular}{lc}

    \hline
    SM diphoton process [fb]  &  1.555 $\pm$ 0.002 \\
    \hline
    \multirow{2}{*}{ADD scenario}            &    Total cross section times \\
    &    branching ratio to two photons [fb] \\
    \hline
     $\ms=3500$~\GeV &   16.47  $\pm$  0.07  \\
     $\ms=4000$~\GeV &   8.60  $\pm$  0.04  \\
     $\ms=4500$~\GeV &   5.09  $\pm$  0.02  \\
     $\ms=5000$~\GeV &   3.44  $\pm$  0.01  \\
     $\ms=5500$~\GeV &   2.58  $\pm$  0.01  \\
     $\ms=6000$~\GeV &   2.159  $\pm$  0.002  \\
     $\ms=6500$~\GeV &   1.927  $\pm$  0.002  \\
     $\ms=7000$~\GeV &   1.797  $\pm$  0.002  \\
     $\ms=7500$~\GeV &   1.716  $\pm$  0.002  \\
     $\ms=8000$~\GeV &   1.667  $\pm$  0.002  \\
    \hline
  \end{tabular}
  \caption{
    Cross section of SM processes producing two prompt photons,
    and cross section times branching ratio to two photons in the presence of ADD model
    calculated at leading order using \textsc{Sherpa} for different values of the ADD model parameter \ms\ in the GRW formalism. The uncertainties correspond to the statistical uncertainties.
    In all the calculations, the following requirements are included in \textsc{Sherpa}: both photons with $\et > 5$~\GeV, $\Delta R$ between the two photons larger than 0.2, $\mgg > 1800$~\GeV. In addition, the Frixione isolation (Phys. Lett. B 429 (1998) 369) for both photons satisfies $\delta_0 = 0.3$, exponent $n = 2$, $\epsilon = 0.025$.
  }
  \label{tab:add_xsection}
\end{table}

\begin{table}
  \centering
  \begin{tabular}{lcc}
    \multirow{2}{*}{Selection}            &    Efficiency & Efficiency \\
    &    ($\ms=3500$~\GeV) & ($\ms=6000$~\GeV) \\
    \hline
    Skimming (including trigger)  &  93\% & 95\% \\[3mm]
    Two photons passing basic shower shape & \multirow{2}{*}{81\%} & \multirow{2}{*}{83\%} \\
    requirements and fiducial selection   & & \\[3mm]
    Trigger matching & 81\% & 82\% \\[3mm]
    Photon identification & 70\% & 70\% \\[3mm]
    Photon isolation & 67\% & 66\% \\[3mm]
    $\mgg>2240$~\GeV & 46\% & 51\% \\[3mm]
    Photon $\et > 55$~\GeV & 46\% & 51\% \\[3mm]
    \hline
  \end{tabular}
  \caption{Selection efficiency (in percentage) for simulated ADD events after each event selection requirement in the spin-2 non-resonant search.
    The SM expectation has been subtracted from all the calculations.
    The simulated \textsc{Sherpa} samples include the following event-generator-level requirements: both photon \et\ larger than 5~\GeV, $\Delta R$ between the two photons larger than 0.2, $\mgg > 1800$~\GeV. In addition, the Frixione isolation (Phys. Lett. B 429 (1998) 369) for both photons satisfies $\delta_0 = 0.3$, exponent $n = 2$, $\epsilon = 0.025$.
  }
  \label{tab:cutflow}
\end{table}
